# Supplementary material for: Projection of Functionals and Fast Pricing of Exotic Options
Source: arXiv:2111.03713 source file (2022-04-29)
Supplement: Supplementary file 1 [file Appendix.tex]

\newpage
\subsubsection{Covariance Kernel of Running Maximum}

\begin{proposition}
The covariance kernel is given by 
$$\kappa_Y(s,t)=  \frac{s}{2} + \frac{\sqrt{s(t-s)}- 2\sqrt{st} + t \,\textnormal{arcsin}(\sqrt{s/t})}{\pi}$$
\end{proposition}

\begin{proof}
Let $\tau_t$ be  the last time the maximum of $X$ has been reached in $[0,t]$ (the optimal time—ex-post—to sell if $X$ is seen as a stock process).  Note that  $\tau_t$ is also the last visit  of $Y-X$  to the origin, i.e. 
$$\tau_t = \sup \calN_t^{Y-X}, \quad \calN_t^{W} = \{s \in [0,t] \, | \, w_s = 0 \}.$$
Now since $y_t - x_t \overset{d}{=} |x_t|$ and 
$\calN_t^{|X|} = \calN_t^{X}$, \rr{then $ \tau_t \overset{d}{=} \sup \calN_t^{X}$}. The distribution of the latter is known, and finally gives
$$\Q(\tau_t\le s) = \frac{2}{\pi} \textnormal{arcsin}(\sqrt{s/t}). \qquad (?)$$

Idea: Fix $s\le t$:
\begin{enumerate}
    \item 
\begin{align*}
    \E[y_s y_t] &= \frac{ \E[y_t^2] + \E[y_s^2] - \E[(y_t - y_s)^2] }{2}
\end{align*}
and use $\E[(y_t - y_s)^2]=\E[(y_t - y_s)^2\mathds{1}_{\{\tau_t \le s\}}]$
\item 
\begin{align*}
    \E[y_s y_t] &= \E[y_s y_t\mathds{1}_{\{\tau_t \le s\}}] + \E[y_s y_t\mathds{1}_{\{\tau_t > s\}}]\\\\
   \E[y_s y_t\mathds{1}_{\{\tau_t \le s\}}]  &= \E[y^2_s\mathds{1}_{\{\tau_t \le s\}}] = \E[y^2_t\mathds{1}_{\{\tau_t \le s\}}]\\\\
   \E[y_s y_t\mathds{1}_{\{\tau_t > s\}}] &= \E[y_s y_{s,t}\mathds{1}_{\{\tau_t > s\}}] = \E[y_s (x_s + \tilde{y}_{t-s})\mathds{1}_{\{\tau_t > s\}}]
\end{align*}

\item Local time approach: $y_t = x_0 + \frac{1}{2}l_t^{Y-X}(0)$, so that ($x_0=0$)
$$y_t = \frac{1}{2}l_s^{Y-X}(0) + \frac{1}{2}l_{s,t}^{Y-X}(0) \overset{\text{Markov}}{=} y_s + x_s + \frac{1}{2}l_{t-s}^{\tilde{Y}-\tilde{X}}(0). $$
Thus, 
\begin{align*}
    \E[y_s y_t] &= \E[y_s^2] + \E[y_s x_s] + \frac{1}{2} \E[y_s] \E[l_{t-s}^{\tilde{Y}-\tilde{X}}(0)]\\
    &= s + \E[y_s x_s] + 2\frac{\sqrt{s(t-s)}}{\pi}
\end{align*}

Note that 
$$s = \E[|x_s|^2] = \E[(y_s - x_s)^2] = \E[y_s^2] + \E[x_s^2] - 2 \E[y_s x_s] \, \Longrightarrow \E[y_s x_s] = \frac{s}{2}.$$

Hence, $\E[y_s y_t] = \frac{3s}{2}  + 2\frac{\sqrt{s(t-s)}}{\pi}$.

\end{enumerate}

\end{proof}
